# Supplementary material for: SP3D: Boosting Sparsely-Supervised 3D Object Detection via Accurate Cross-Modal Semantic Prompts
Source: arXiv:2503.06467 source file (2025-03-09)
Supplement: Supplementary file 2 [file X_suppl.tex]

\maketitlesupplementary
